# Supplementary material for: Sensitive Dependence of Global Climate to Continental Geometry
Source: arXiv:2205.15089 source file (2022-05-30)
Supplement: Supplementary file 1 [file supplement.pdf]

# Supporting Information for "Sensitive Dependence of Global Climate to Continental Geometry"

Mark Baum[1], Minmin Fu[1], and Stephen Bourguet[1]

[1]Harvard University, 20 Oxford St., Cambridge MA 02138

**Contents of this file**

1. Text S1

2. Table S1

**Text S1.**

## 1. Synthetic Continental Configurations

Continental configurations are generated using randomized, truncated spherical harmonic expansions. Like any spectral basis, spherical harmonics exhibit finer structure at higher degrees. Expansions with more weight on high degrees appear more broken-up and vice versa. To create a random continental configuration, we generate random coefficients for an expansion truncated at degree 12 and reduce the coefficients in each degree so that the expansion satisfies the proportionality

$$S \propto d^p \,, \tag{1}$$

where $S$ is the sum of squared coefficients in each degree, $d$ is the expansion degree, and $p$ defines the "color" of the expansion as in traditional signal processing.

The value of $p$ determines the balance between low and high degree harmonics. For $p = -3$, high frequency terms are suppressed and the expansion has a consolidated structure resembling a supercontinent. For $p = -2$, the balance shifts away from low degrees and the supercontinent has started breaking up. For $p = -1$, higher degree harmonics become apparent, resembling a rifted/broken-up continental configuration. By adjusting the same set of initial random coefficients for $p \in \{-3, -2, -1\}$, we acquire expansions which differ in the weight of each degree but not the relative values within each degree. The similarity within each degree preserves the basic structure across values of $p$, representing discrete snapshots along the breakup of a supercontinent.

After generating expansion coefficients with the desired $p$ value, we evaluate the expansion on a $0.5° \times 0.5°$ grid. We then enforce a given land fraction $\gamma$ numerically by finding the elevation $z_\gamma$ such that the area of cells exceeding $z_\gamma$ is closest to $\gamma A$, where $A$ is the Earth's surface area. Cells above $z_\gamma$ are land and cells below $z_\gamma$ are ocean.

Ocean cells are assigned a final elevation of -100 m for interpretation by the GCM. This value is not ultimately relevant because we use a slab ocean. Land cells are each assigned an elevation of +100 m with a small additional contribution proportional to their minimum distance from the ocean. This contribution gives landmasses a very slight convex shape on top of the baseline elevation of 100 m. Convexity is necessary for the GCM to properly route runoff away from the continents. However, the total elevation range across land areas is only tens of meters. This is so small compared to the horizontal

scale of the landmasses that the continents can be thought of as flat, as in previous GCM studies of continental break-up (Donnadieu et al., 2004, 2006).

## 2. GCM configuration

We use the National Center for Atmospheric Research (NCAR) Community Earth System Model (CESM) version 1.2.2.1 with the Community Atmosphere Model (CAM) version 4 as its atmospheric component (Neale et al., 2012). The land component used is the Community Land Model (CLM) version 4.0 (Lawrence et al., 2011). We set obliquity to 23.5° and eccentricity to zero. Land type is set to bare ground for continental regions and all simulations are run using the spectral-element core at T31 resolution (∼4° horizontal resolution) with 26 vertical levels. Each simulation is run for 110 years, with the first 30 years discarded to allow for model spin-up. The ocean component is a slab ocean of 50 m depth, with no prescribed ocean heat transport.

## 3. Global Weathering Estimation

Earth's atmospheric $CO_2$ concentration is thought to be strongly regulated by the carbonate-silicate weathering feedback first proposed by (Walker et al., 1981), with the original author's initials forming the abbreviation "WHAK". A more recent study by (Maher & Chamberlain, 2014), also abbreviated using author initials as "MAC," introduced a revised framework for understanding silicate weathering where temperature plays a weaker role than in the WHAK model.

### 3.1. The WHAK Model

In the original WHAK model, silicate weathering was parameterized using

$$w \propto qp^{\beta}e^{(T-T_0)/T_c}\,, \tag{2}$$

where $q$ is the rate of river runoff, $p$ is the $CO_2$ partial pressure, $\beta$ is a parameter representing the effect of $p$ on cation dissolution, $T_0$ is a reference temperature, and $T_c$ is a constant derived from laboratory experiments that represents differences in cation concentration for reactions occurring under different temperature conditions (Lagache, 1976). The runoff $q$ was further parameterized as a function of $T$, based on numerical climate simulations indicating that $q \propto e^{(T-T_0)/60\mathrm{K}}$ (Manabe & Wetherald, 1975). Incorporating this temperature dependence of river runoff and cation dissolution gives the following estimate of global silicate weathering rate as a function of $p$ and $T$,

$$W/W_0 = (p/p_0)^{\beta}e^{(T-T_0)/T_e}\,, \tag{3}$$

where $W_0$ is an estimate of the present-day rate of silicate weathering (Gerlach, 2011; Haqq-Misra et al., 2016) and $p_0$ is the pre-industrial $CO_2$ partial pressure.

In the WHAK model, the silicate weathering feedback stabilizes Earth's climate via two negative feedback mechanisms, one involving the increase in rainfall and hence runoff ($q$) with warming, and the second due to the enhancement of kinetic weathering rate as a function of increasing global temperature. The latter process, however, is dominant in the WHAK model based on the much weaker temperature dependence of the runoff term. Variations of the WHAK model have been used in numerous studies of climate evolution and habitability. Some studies have included the direct $pCO_2$ dependence term (Abbot et al., 2012), while others have omitted it (Goddéris et al., 2017).

For application to spatially resolved climate simulations, where runoff is explicitly simulated rather than parameterized as a function of temperature, we write the WHAK weathering rate as

$$w = kq \left( \frac{p}{p_0} \right)^{\beta} \exp \left( \frac{T - T_0}{T_e} \right) . \quad (4)$$

Global weathering is calculated by summing over all cells of the simulation,

$$W = \sum_i A_i f_i w_i \, , \quad (5)$$

where $i$ indicates the $i^{\text{th}}$ grid cell, $A_i$ is the surface area of the cell, $f_i$ is the cell's land fraction, and $w_i$ is computed using Equation 4. The calibration constant $k$ is 0.18, identical for all cells. The WHAK model must always be calibrated and this value yields global weathering rates in the vicinity $7 \times 10^{12}$ mol/yr, a reasonable estimate for the global $CO_2$ outgassing rate. Parameter values used in this study are given in Table S1.

### 3.2. The MAC Model

Maher and Chamberlain (Maher & Chamberlain, 2014) introduced a revised framework for understanding silicate weathering where temperature plays a weaker role than originally proposed in the WHAK model. The MAC model represents a more complete set of physical processes and incorporates a maximum concentration for weathering products $C_{\text{eq}}$, thus imposing a "thermodynamic limit" on chemical weathering rates. For the purposes of our study, we closely followed the derivation of (Graham & Pierrehumbert, 2020).

Key to the MAC model is the Damköhler number ($D$), a non-dimensional parameter which represents the ratio between the mean fluid travel time ($T_f \approx L\phi q$) to the timescale to reach chemical equilibrium ($T_{\text{eq}} \approx C_{\text{eq}}/R$), where $q$ is runoff, $L$ is flow-path length, $\phi$

is effective porosity, $C_{\text{eq}}$ is the maximum solute concentration, and $R$ is the reaction rate. Reactivity is written as $R = R_{\max} f_w$, where $f_w = (X_s/X_r)$ is the fresh mineral fraction. $f_w$ is parameterized as $(1 + mk_{\text{eff}}At_s)^{-1}$, where $A$ is the specific surface area, $m$ is the mineral molar mass, $k_{\text{eff}}$ is a reference weathering rate constant, and $t_s$ is the soil age, reflecting declining reactivity with increasing soil age. By factoring out the runoff ($q$), the Damköhler coefficient ($D_w = Dq$) can be written as

$$D_w = \frac{L\phi\rho_{sf}k_{\text{eff}}AX_r}{C_{\text{eq}}\left(1 + mk_{\text{eff}}t_s\right)}\,, \tag{6}$$

where $C_{\text{eq}}$ represents the maximum cation concentration set by the equilibration between dissolving silicates and precipitating clays (Alekseyev et al., 1997; Maher et al., 2006, 2009; Winnick & Maher, 2018). Furthermore, following (Winnick & Maher, 2018), $C_{\text{eq}}$ is a considered to be a function of atmospheric $\text{pCO}_2$,

$$C_{\text{eq}} = \Lambda\left(\text{pCO}_2\right)^n\,, \tag{7}$$

where $n$ is an exponent derived from a theoretical silicate dissolution and clay precipitation reaction (Winnick & Maher, 2018; Graham & Pierrehumbert, 2020) and $\Lambda$ is a scaling coeffient that depends on the reaction equilibrium constant and stoichiometry (Winnick & Maher, 2018). Note that $C_{\text{eq}}$, as written in Equation 6, has units of mol/L and must be converted to units of mol/kg$^3$ by multiplying by the density of water (1000 kg/L) prior to use in Equation 7. An equation for the MAC weathering rate as function of $D_w$ and $C_{\text{eq}}$ (derived in the supplement of (Maher & Chamberlain, 2014)) can be written as follows.

$$\begin{aligned} w &= qC_{\text{eq}}\frac{\mu D_w/g}{1 + \mu D_w/q} \\ &= \frac{\alpha}{\left[k_{\text{eff,ref}}\exp\left(\frac{T-T_0}{T_e}\right)\left(\frac{p}{p_0}\right)^{\beta}\right]^{-1} + mAt_s + \alpha\left[(qC_{\text{eq}})\right]^{-1}} \end{aligned} \tag{8}$$

where $\alpha \equiv L\phi\rho_s f A X_r \mu$, defined for convenience. The MAC weathering rate is mainly determined by $C_{\mathrm{eq}}$ and $D_w$, which themselves contain many physical parameters (Table S1). We remark that MAC weathering rates are meant to be absolute and are not directly calibrated as WHAK weathering is. However, the default parameters of (Graham & Pierrehumbert, 2020) yield a weathering rate of $2.3\times10^{12}$ mol/yr for our reference simulation, which is below typical estimates of modern-day volcanic outgassing of $7.5 \times 10^{12}$ mol/yr (Gerlach, 2011). Therefore, we slightly modify the MAC parameters by using the higher value of $\Lambda = 0.0084$ that appears in (Winnick & Maher, 2018), and tuning $L$ from 1 m to 1.5 m such that MAC weathering is closer to $7.5 \times 10^{12}$ mol/yr, the assumed value of modern volcanic outgassing.

To apply the MAC model to spatially resolved climate simulations, we use the same cell-by-cell summation expressed in Equation 5, but replacing $w_i$ with the result of Equation 8 for each cell.

## References

Abbot, D. S., Cowan, N. B., & Ciesla, F. J. (2012). Indication of insensitivity of planetary weathering behavior and habitable zone to surface land fraction. *The Astrophysical Journal*, *756*(2), 178.

Alekseyev, V. A., Medvedeva, L. S., Prisyagina, N. I., Meshalkin, S. S., & Balabin, A. I. (1997). Change in the dissolution rates of alkali feldspars as a result of secondary mineral precipitation and approach to equilibrium. *Geochimica et Cosmochimica Acta*, *61*(6), 1125–1142.

Donnadieu, Y., Goddéris, Y., Pierrehumbert, R., Dromart, G., Fluteau, F., & Jacob, R. (2006). A GEOCLIM simulation of climatic and biogeochemical consequences of Pangea breakup. *Geochemistry, Geophysics, Geosystems*, *7*(11).

Donnadieu, Y., Goddéris, Y., Ramstein, G., Nédélec, A., & Meert, J. (2004). A 'snowball Earth' climate triggered by continental break-up through changes in runoff. *Nature*, *428*(6980), 303–306.

Gerlach, T. (2011). Volcanic versus anthropogenic carbon dioxide. *Eos, Transactions American Geophysical Union*, *92*(24), 201–202.

Goddéris, Y., Donnadieu, Y., Carretier, S., Aretz, M., Dera, G., Macouin, M., & Regard, V. (2017). Onset and ending of the late Palaeozoic ice age triggered by tectonically paced rock weathering. *Nature Geoscience*, *10*(5), 382–386.

Graham, R. J., & Pierrehumbert, R. (2020). Thermodynamic and energetic limits on continental silicate weathering strongly impact the climate and habitability of wet, rocky worlds. *The Astrophysical Journal*, *896*(2), 115.

Haqq-Misra, J., Kopparapu, R. K., Batalha, N. E., Harman, C. E., & Kasting, J. F. (2016). Limit cycles can reduce the width of the habitable zone. *The Astrophysical Journal*, *827*(2), 120.

Lagache, M. (1976). New data on the kinetics of the dissolution of alkali feldspars at 200 °C in $CO_2$ charged water. *Geochimica et Cosmochimica Acta*, *40*(2), 157–161.

Lawrence, D. M., Oleson, K. W., Flanner, M. G., Thornton, P. E., Swenson, S. C., Lawrence, P. J., ... Slater, A. G. (2011). Parameterization improvements and functional and structural advances in Version 4 of the Community Land Model. *Journal of Advances in Modeling Earth Systems*, *3*(1).

Maher, K., & Chamberlain, C. P. (2014). Hydrologic regulation of chemical weathering and the geologic carbon cycle. *Science*, *343*(6178), 1502–1504.

Maher, K., Steefel, C. I., DePaolo, D. J., & Viani, B. E. (2006). The mineral dissolution rate conundrum: Insights from reactive transport modeling of U isotopes and pore fluid chemistry in marine sediments. *Geochimica et Cosmochimica Acta*, *70*(2), 337–363.

Maher, K., Steefel, C. I., White, A. F., & Stonestrom, D. A. (2009). The role of reaction affinity and secondary minerals in regulating chemical weathering rates at the Santa Cruz Soil Chronosequence, California. *Geochimica et Cosmochimica Acta*, *73*(10), 2804–2831.

Manabe, S., & Wetherald, R. T. (1975). The effects of doubling the $CO_2$ concentration on the climate of a general circulation model. *Journal of Atmospheric Sciences*, *32*(1), 3–15.

Neale, R. B., Chen, C.-C., Gettelman, A., Lauritzen, P. H., Park, S., Williamson, D. L., ... others (2012). Description of the NCAR community atmosphere model (CAM 5.0). *NCAR Tech. Note NCAR/TN-486+ STR*.

Walker, J. C. G., Hays, P. B., & Kasting, J. F. (1981). A negative feedback mechanism for the long-term stabilization of Earth's surface temperature. *Journal of Geophysical Research: Oceans*, *86*(C10), 9776–9782.

Winnick, M. J., & Maher, K. (2018). Relationships between $CO_2$, thermodynamic limits on silicate weathering, and the strength of the silicate weathering feedback. *Earth and Planetary Science Letters*, *485*, 111–120.

**Table S1.** Parameter values and units used in the WHAK and MAC weathering. These parameters are used in Equations 4 and 8. The Units column is left blank for dimensionless quantities.

| Parameter | Description | Value | Unit |
|---|---|---|---|
| $k$ | WHAK calibration constant | 0.18 | $mol/m^3$ |
| $p_0$ | reference $pCO_2$ | $285 \times 10^{-6}$ | bar |
| $\beta$ | pCO2 scaling | 0.2 | |
| $T_0$ | reference temperature | 288.15 | K |
| $T_e$ | temperature scaling | 11.1 | K |
| $n$ | thermodynamic $pCO_2$ dependence | 0.316 | |
| $\Lambda$ | thermodynamic coefficient for $C_{\mathrm{eq}}$ | 0.0084 | |
| $L$ | flow path length | 1.5 | m |
| $\phi$ | porosity | 0.1 | |
| $\rho$ | mineral mass to fluid volume ratio | 12728 | $kg/m^3$ |
| $k_0$ | reference rate constant | $8.7 \times 10^{-6}$ | $mol/m^2/yr$ |
| $A$ | specific surface area | 100 | $m^2/kg$ |
| $X$ | reactive mineral concentration | 0.36 | |
| $t_s$ | soil age | $10^5$ | yr |
| $m$ | mineral molar mass | 0.27 | kg/mol |
| $\mu$ | scaling constant | $e^2$ | |
